# Supplementary material for: Suppression of dephasing by qubit motion in superconducting circuits
Source: arXiv:1509.00122 source file (2015-09-01)
Supplement: Supplementary file 1 [file supplemental_material.pdf]

# Suppression of dephasing by qubit motion in superconducting circuits

D. V. Averin[1],[*] K. Xu[2], Y. P. Zhong[2], C. Song[2], H. Wang[2],[†] and Siyuan Han[3‡]
[1]*Department of Physics and Astronomy, Stony Brook University, SUNY, Stony Brook, NY 11794-3800, USA*
[2]*Department of Physics, Zhejiang University, Hangzhou, Zhejiang 310027, China*
[3]*Department of Physics and Astronomy, University of Kansas, Lawrence, KS 66045, USA*
(Dated: August 30, 2015)

Online supplementary material to the paper Suppression of dephasing by qubit motion in superconducting circuits.

## THE HIGH-FREQUENCY CUTOFF $\omega_h$

In the main text, we presented the theory result for the suppression of the $1/f$ noise, given by the Eqs. (6) and (7) with the noise intensity $W_j^2 = (A_j/\pi)\ln(\omega_h/\omega_l)$, in the situation when the high-frequency cutoff $\omega_h$ of the $1/f$ noise is sufficiently low, i.e., satisfies the condition $\omega_h \ll n/\tau$. Here we want to briefly point out that the main result, Eq. (7), predicting the $\sqrt{n}$ increase of the dephasing time due to qubit motion remains valid, up to a weak logarithmic correction, also for the large high-frequency cutoff which satisfies the condition $\omega_h \gg n/\tau$. In this regime, the full integral for the qubit dephasing in Eq. (5) converges at high frequencies and does not require the high-frequency cutoff:

$$F(\tau) = \exp\{-\frac{2}{\pi}\sum_{j=1}^{n} A_j \int_{\omega_l}^{\infty} d\omega \frac{\sin^2(\omega\tau/2n)}{\omega^3}\}\,. \qquad \text{(S1)}$$

Evaluating the integral in this expression with logarithmic accuracy, and assuming that the noise intensities in all physical qubits are the same, $A_j = A$, we find

$$F(\tau) = \exp\{-\tau^2 \frac{A}{2\pi n} \ln \frac{2n}{\omega_l \tau}\}\,. \qquad \text{(S2)}$$

This result is different from the one given in Eq. (7) of the main text only in that the role of the high-frequency cutoff $\omega_h$ under the logarithm is played by the factor $2n/\tau$, making the effective dephasing time $\tau_d$ weakly dependent of the real time $\tau$ through the logarithm in Eq. (S2).

## SYNTHESIZING ARTIFICIAL NOISES

Dephasing can be treated as resulting from an ensemble average of many trajectories during which the qubit motion accumulates random phases. To inject artificial flux noise and imitate the qubit's $1/f$ noise environment, we apply the specifically-designed series of bias sequences in the Ramsey fringe measurements and average the outcomes, from which the dephasing time can be estimated. Each bias sequence consists of successive 4-ns-wide square pulses, whose amplitudes are set by the following procedure such that the time series of all these amplitude values (from all bias sequences) yield the desired flux-noise power spectrum, e.g., $S_j^E(\omega) \propto 1/\omega$ for qubit $j$. To proceed, we first discretize the desired spectrum function $S_j^E(\omega)$ into the series $S_j^E(\omega_m)$, where $\omega_m = 2\pi m/(Nk\tau_0)$ $(m = 0, 1, 2, \ldots, Nk/2)$ and $\tau_0 = 4$ ns. Here $N$ is the number of bias sequences and $k$ is the maximum number of the 4-ns-wide square pulses for each bias sequence ($k\tau_0$ is therefore the maximum time for each Ramsey fringe curve). We then multiply $\sqrt{S_j^E(\omega_m)}$ by a phase factor $\theta_m$ that is randomly chosen between 0 and $2\pi$. Subsequently we perform the inverse Fourier transform of the series $\left\{\sqrt{S_j^E(\omega_m)}\exp(i\theta_m),\, m = 0, 1, 2, \ldots, Nk/2\right\}$ to generate the desired time series $\xi$ that consists of $Nk$ numbers (Fig. S1(a)) [1]. The time series $\xi$ is then split into $N$ sections. Each of the $N$ sections corresponds to a single bias sequence, and in each section the $k$ numbers are transformed to the square pulses' amplitudes as experimentally realized by an arbitrary waveform generator (Fig. S1(b)). We have numerically verified that noise generated in this manner have the desired $1/f$ spectrum over the frequency range $[1/(Nk\tau_0), 1/(2\tau_0)]$.

We test our protocol of generating artificial noises using a circuit consisting of two Xmon qubits coupled to a common resonator. The resonator frequency $\omega^r/2\pi = 5.11$ GHz and the qubit-resonator coupling strength $\lambda/2\pi \approx 23$ MHz. We tune the resonant frequencies of the two Xmon qubits to 5.34 and 5.59 GHz, respectively, where both Xmon qubits have the energy relaxation time $T_1 \approx 10$ $\mu$s and the dephasing time $T_2^* \approx 800$ ns in absence of the artificial noise, where $T_2^*$ is estimated assuming that the Ramsey envelope decays as $\exp\left[-\tau/2T_1 - (\tau/T_2^*)^2\right]$. For each of the two qubits, the $k$ square pulses with varying amplitudes in a single bias sequence shift the qubit resonant frequency and thus disturb the oscillations of the $|1\rangle$-state population ($P_1$) in a Ramsey fringe curve (Fig. S2(a)). For example, averaging $N = 100$ Ramsey fringe curves measured under the artificial noise sequences similar to that shown in Fig. S2(a) we obtain the outcome in Fig. S2(b), from which we estimate that $T_2^*$ is reduced to 223 ns due to the injected noise for one of the two qubits.

To explore the effectiveness of the motion qubit method in presence of correlated noises, here we artificially inject two noise sequences with different degrees of

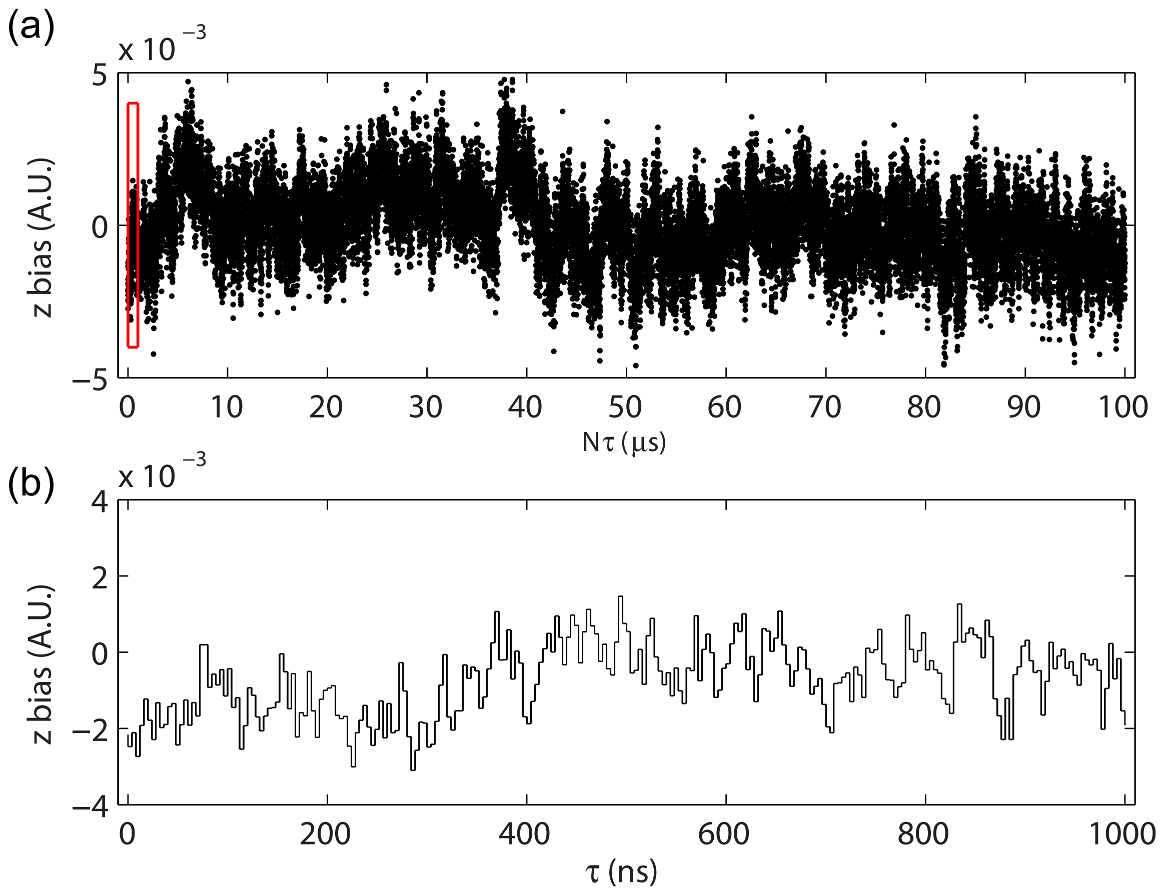


FIG. S1: (a) The $Nk$ numbers generated by the method outlined in text for simulating the $1/f$ noise spectrum, where $N = 100$ and $k = 250$. (b) Zoom-in view of the first $k$ numbers highlighted in the red box in **a** for composing a bias sequence. Each square pulse is 4 ns in width and its amplitude (height) is set by the $k$-number series.

correlations to two Xmon qubits, respectively, based on which the 2-qubit Ramsey fringe measurements are performed to estimate $\tau_d^E$, the logic-qubit dephasing time under artificial (extrinsic) noises. Correlated noises with a given correlation coefficient $r$ are generated using the following procedure. We first generate two independent time series $\xi_1$ and $\xi_2$ with the same power spectrum as outlined previously, based on which we generate a new series $\xi_2' = r\xi_1 + \sqrt{1-r^2}\xi_2$. It can be verified that $\mathrm{corr}(\xi_1, \xi_2') = r$, where $\xi_2'$ has the same power spectrum as that for $\xi_1$ and $\xi_2$. The two noise sequences determined by $\xi_1$ and $\xi_2'$ are then applied to the two Xmon qubits, respectively.

It should be noted that our protocol of simulating the $1/f$ noise spectrum with $N = 100$ and $k = 250$ is only an approximate. To reach the lower frequency limit of the true $1/f$ noise that is relevant to a Ramsey fringe experiment by our simulation protocol, $N$ has to be much larger than 100 so that $1/(Nk\tau_0)$ can reach the order of 1 Hz.

* Electronic address: dmitri.averin@stonybrook.edu
† Electronic address: hhwang@zju.edu.cn
‡ Electronic address: han@kansas.edu

[1] M. J. Biercuk, *et al.* Nature **458**, 996-1000 (2009).

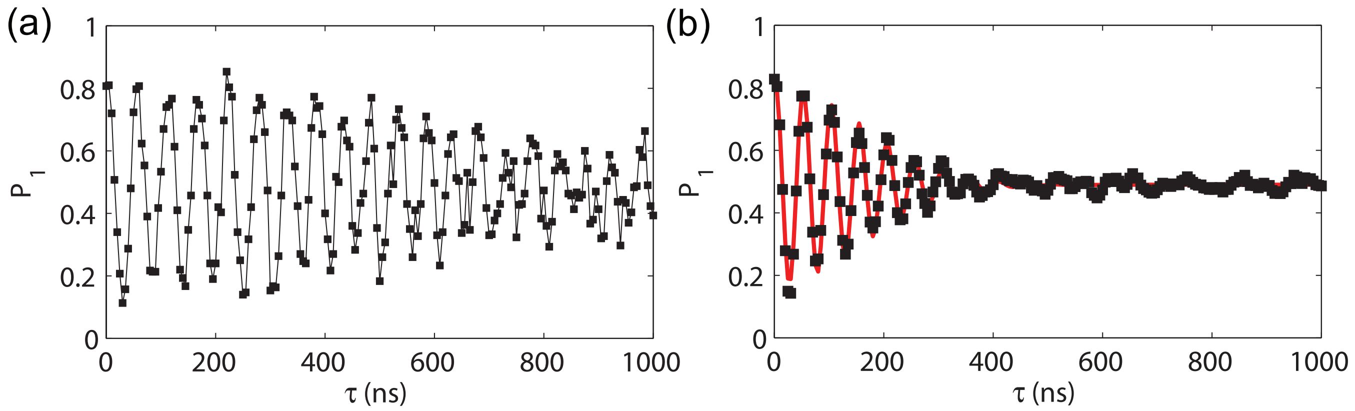


FIG. S2: (a) The Ramsey fringe curve measured under the artificial noise defined by the $k$ numbers in Fig. S1(b). The noise jitter the qubit resonant frequency and thus disturb the oscillations of the $|1\rangle$-state population ($P_1$). (b) Averaged result of the $N = 100$ Ramsey fringe curves measured under the artificial noise defined by the $Nk$ numbers in Fig. S1(a). Dots are the experimental data, and line is a fit. $T_2^*$ is reduced to 223 ns due to the artificial noise.
